# Supplementary material for: Properties of the Be-type stars in 30 Doradus
Source: arXiv:2203.02440 source file (2022-03-07)
Supplement: Supplementary file 1 [file Appendix.pdf]

## APPENDIX A: COMMENTS ON INDIVIDUAL STARS

Four targets were excluded principally due to it not being possible to estimate projected rotational velocities:
#039: The spectrum is dominated by emission lines, precluding any reliable rotational or radial velocity estimates. The position of the Si IV lines near 4100Å varies with epoch, implying binarity.
#689: The spectrum shows narrow absorption lines, together with narrow and broad emission features. However the width of lines in multiplets such as the O II features near 4070Å and 4416Å imply significant rotational broadening, $v_e \sin i \sim 200\,\mathrm{km\,s^{-1}}$.
#766: Evans et al. (2015) assigned a B5-8e spectral type consistent with a weak He I spectrum. As this star has a later spectral type than the rest of the sample it has been excluded from the analysis.
#822: The spectrum contains a plethora of emission features, which mask those from the photosphere. Kalari et al. (2014) assigned a B8[e] spectral type and from optical spectroscopy and infrared photometry suggested that it might be a Herbig B[e] star.

The Hubble Legacy Archive was searched for spatially close companions for the remaining 69 targets, Nine targets (#387, 401, 683, 781, 794, 813, 877, 880, 889) had no suitable imaging. For the remaining targets, fifty two had no companion within the fibre radius (0.6″) and only fainter targets within two fibre radii. The remaining 9 targets showed evidence for possible contamination as follows:
#068: Fainter companion at ∼0.7″.
#272: #271, classified as an A-type supergiant, lies ∼1.2″ away and is approximately 20 times brighter in the V-band (Evans et al. 2011).
#283: Two companions with comparable I band magnitude at ∼0.5″
#287: Three fainter companions within 0.5″
#301: Companion with a similar I band magnitude at ∼1″.
#644: Companion with a similar I band magnitude at ∼0.5″.
#824: Two stars with a comparable I band magnitude lie within the fibre aperture and the spectrum is almost certainly composite.
#835 and #836: These are separated by 1.32″. Their spectroscopy implies significantly different projected rotational velocities, implying that any contamination is small.

Below we comment on 16 targets, mostly a quality rating, Q=3:
#022, #068, #135, #268, #320, #337, #408, #644: Significant nebular contamination in the He I lines, which is particularly strong in the diffuse triplet features. Additionally, there might be some cross fibre contamination for #320 due to a bright target being in an adjacent fibre. The $v_e \sin i$ estimates are restricted to the singlet and non-diffuse lines and often lead to large sample standard deviations. For #644, the estimate from the Mg II doublet is consistent with the moderate $v_e \sin i$ estimate from the He I spectrum,
#272: This spectrum contains many narrow absorption lines, consistent with its close proximity to the bright A-type supergiant, #271. VFTS spectroscopy for #271 could be used to remove its contribution to the composite spectrum, with a flux contribution ∼40% being implied.[4]
#298: The combination of a large $v_e \sin i$, a relative low S/N ratio and significant He I emission limits the number of estimates. However the theoretical profiles are convincing, whilst the sample standard deviation is relatively small.
#322: The He I spectrum is badly affected by nebular emission and only four estimates are possible, leading to $v_e \sin i = 185 \pm 25\,\mathrm{km\,s^{-1}}$. Estimates are also available from four Set 1 lines and yielded a mean value, $v_e \sin i = 166 \pm 11\,\mathrm{km\,s^{-1}}$. We have adopted the latter value given its smaller standard deviation and the lack of contamination from nebular emission.

[4] The S/N ratio listed in Table 2 is for the corrected spectroscopy

**Table B1.** Differences between the $v_e \sin i$ estimates from individual He I lines and the means summarized in Table 2. The mean differences, their standard deviations ($\sigma$) and the number of estimates (n) are summarized for all the targets and for the subset with quality ratings of 1 or 2.

| $\lambda$ | All targets | | | Q=1–2 targets | | |
|---|---|---|---|---|---|---|
| | Mean | $\sigma$ | n | Mean | $\sigma$ | n |
| 4009 | +13 | 23 | 52 | +11 | 22 | 43 |
| 4026 | +3 | 19 | 51 | +2 | 17 | 42 |
| 4121 | -15 | 25 | 40 | -14 | 23 | 34 |
| 4144 | +2 | 26 | 59 | +3 | 23 | 45 |
| 4388 | -9 | 24 | 53 | -9 | 23 | 43 |
| 4471 | +2 | 19 | 26 | +4 | 20 | 23 |
| 4713 | +1 | 20 | 18 | +1 | 20 | 18 |
| 4922 | -2 | 22 | 17 | -3 | 22 | 16 |

#395: The moderate S/N leads to the observations of the Set 1 lines being relatively poor. However the different estimates are in reasonable agreement, whilst the clear separations of the O II doublet at approximately 4417Å and of the lines near 4070Å are consistent with the adopted $v_e \sin i$. Evans et al. (2015) identified some cross-fibre contamination from the Wolf-Rayet star, RMC 135 (#402)
#781: This spectrum contains broad emission features, whilst there may be shell like absorption in the cores of the He I. Additionally the individual estimates show considerable scatter. The identification of C II and Si III lines supports the relatively small $v_e \sin i$ estimate.
#824 and #840: These two targets have the lowest S/N (∼45) of our sample and there is nebular emission in some of the He I lines. However the identification of the C II and Mg II doublets implies a relatively small projected rotational velocity for #824.
#854: The spectroscopy for this target also has a relatively low S/N and the He I spectrum is intrinsically weak.

## APPENDIX B: STOCHASTIC UNCERTAINTIES IN $v_e \sin i$ ESTIMATES

The estimation of projected rotational velocities for Be-type stars is complicated by the nature of their spectra. Here we consider their reliability assuming that the adopted methodologies are valid. This assumption is considered further in Sect. 3.2.

The majority (∼80%) of the $v_e \sin i$ estimates were obtained with the line-set 2 and we have searched for differences between the estimates obtained from different lines.[5] In Table B1, the systematic offset, its standard deviation and number of estimates for each line are summarized. Offsets are provided both for all targets and for the subset excluding the Q=3 estimates; in general slightly better agreement is found for the latter as would be expected.

The agreement is excellent for 5 lines (at 4026, 4143, 4471, 4713 and 4922 Å) with absolute systematic offsets of less than $5\,\mathrm{km\,s^{-1}}$. For the other lines, the differences are larger and in the range of 9–15 $\mathrm{km\,s^{-1}}$. The He I line at 4009 Å is the weakest and broadest of the 6 diffuse features. As such the larger $v_e \sin i$ estimates obtained from this line may reflect the greater intrinsic broadening relative to the rotational broadening. The non-diffuse He I line at 4121 Å lies in the red wing of a Balmer line, which may have lead to its normalisation

[5] Only 10 targets were analysed using Set 1. The systematic offsets for all these lines are less than $5\,\mathrm{km\,s^{-1}}$ and none of them are statistically significant.

**Table B2.** Comparison of the projected rotational velocity estimates obtained from the two line-sets. The results for set 2 have been taken directly from Table 2.

| VFTS | Set 2 estimate | | | | Set 1 estimate | | |
|---|---|---|---|---|---|---|---|
| | $v_e \sin i$ | $\sigma$ | $n$ | Q | $v_e \sin i$ | $\sigma$ | $n$ |
| 034 | 174 | 15 | 8 | 1 | 182 | 22 | 4 |
| 166 | 227 | 29 | 8 | 1 | 213 | – | 1 |
| 194 | 217 | 28 | 6 | 1 | 203 | 26 | 2 |
| 196 | 200 | 9 | 6 | 1 | 190 | 6 | 3 |
| 200 | 260 | 12 | 7 | 1 | 240 | – | 1 |
| 213 | 181 | 20 | 6 | 1 | 163 | 16 | 5 |
| 283 | 279 | 20 | 8 | 1 | 270 | 2 | 2 |
| 301 | 260 | 19 | 7 | 1 | 242 | 15 | 3 |
| 330 | 248 | 10 | 7 | 1 | 263 | 25 | 3 |
| 401 | 261 | 13 | 6 | 1 | 261 | 24 | 3 |
| 644 | 187 | 13 | 3 | 3 | 196 | – | 1 |
| 685 | 276 | 15 | 5 | 2 | 260 | – | 1 |
| 738 | 190 | 13 | 6 | 1 | 197 | 15 | 3 |
| 794 | 274 | 13 | 7 | 1 | 272 | 2 | 2 |
| 796 | 189 | 19 | 6 | 1 | 175 | 23 | 2 |
| 813 | 213 | 24 | 6 | 1 | 221 | 13 | 2 |
| 836 | 221 | 15 | 6 | 1 | 200 | 11 | 2 |
| 848 | 150 | 6 | 6 | 1 | 146 | 12 | 4 |

being less reliable. By contrast the estimates for the other non-diffuse line (at 4713 Å) show no significant offset from the mean estimates.

The cause of the offset for the line at 4388 Å is unclear, as it is well observed, and has neither especially strong wings and does not suffer from strong nebular emission. Dufton et al. (2013) estimated projected rotational velocities for the VFTS B-type targets that were apparently single (Dunstall et al. 2015), using the same Fourier Transform methodology. Excluding the Be-type stars, estimates from the He I spectrum were available for 165 targets, leading to a mean offset for the 4388 Å of -9±20 km s$^{-1}$. This is very similar to that in Table B2 and implies that the systematic difference is not due to the Be-type nature of our sample. Excluding estimates from this line would have increased the mean $v_e \sin i$estimates by $\lesssim$2 km s$^{-1}$.

The observed profiles for our target can be compared with theoretical profiles that include rotational broadening. Agreement is generally satisfactory in the line centres but the observed profiles often have more extended wings particularly for the He I diffuse lines, as illustrated in Fig. B1. This is consistent with the theoretical profiles excluding any contribution from the intrinsic profile. To investigate this, we have extracted theoretical stellar spectra for the atmospheric parameters of #034 listed in Table 4 using the grid of models discussed in Sect. 5. The observed and theoretical profiles for #034 (convolved with a broadening function for $v_e \sin i$=175 km s$^{-1}$) are shown in Fig. B1. The agreement between the observed and theoretical spectra is now reasonable both in the line core and in the wings. This illustrates one of the strengths of the FT methodology, viz. that it can identify the signature of rotational broadening even in the presence of complex intrinsic line profiles.

For each target, a line-set was chosen depending on the visibility of the corresponding spectral features. However for some of the targets (with $v_e \sin i \lesssim$280 km s$^{-1}$) where the line-set 2 had been adopted, metal lines from line-set 1 could also be analysed. Table B2 summarizes these measurements together with the estimates from line-set 2, taken directly from Table 2. Generally good agreement is found between the two sets of measurements with a mean offset (line-set 1 - line-set 2) of -7±12 km s$^{-1}$ is found. This is marginally statistically significant assuming a normal error distribution and may reflect the larger intrinsic widths of the He I diffuse lines in line-set 2. However this comparison is encouraging although inevitably it does not include any of the larger $v_e \sin i$ estimates.

Two methodologies were adopted in obtaining $v_e \sin i$ estimates, viz. searching for minima in the Fourier Transform and least-squares fitting of the line profiles. As the latter does not take account of the instrumental broadening or the intrinsic line profile, it may lead to overestimates especially for the diffuse He I lines. Using the results of Dufton et al. (2013) for the 165 apparently single non-Be type stars, we find a mean and standard deviation for the ratios of the PF to the FT estimates of R=1.06±0.05. For the current line-set 2 estimates of 59 targets, a ratio R=1.02±0.05 is found. The better agreement between the two methodologies in this case is probably due to the Be-type sample having on average larger $v_e \sin i$estimates, thereby reducing the importance of other broadening mechanisms.

Previously Dufton et al. (2013) and Garland et al. (2017) used the FT methodology to estimate projected rotational velocities for the apparently single and SB1 VFTS targets respectively. A comparison of their results with those obtained here is shown in Fig. B2. The agreement is generally good with a mean ratio of 0.98±0.07. For only one star, #824, is the difference more than 20% and as discussed in Appendix A, the S/N of this star is low and the estimate has a quality rating, Q=3. Six additional targets have estimates that differ by more than 10%. Four (#068, #156, #337, #735) again have quality ratings, Q=2–3 and the difference between the estimates is not statistically significant, whilst #237 (Q=1) has a low $v_e \sin i$ estimate and the difference of 16 km s$^{-1}$is again consistent with the estimated errors. For the final target, #786 (Q=1), the current estimate is approximately 40 km s$^{-1}$larger at 314 km s$^{-1}$. The estimates for individual lines from the two analyses are in reasonable agreement apart from that for the He I at 4922 Å, where Dufton et al. (2013) found an anomalously low value of 230 km s$^{-1}$. Excluding this measurement would reduce the discrepancy to 8%.

The error estimates on our $v_e \sin i$ estimates are on average 20% lower than those of Dufton et al. (2013) and Garland et al. (2017). This probably reflects a more careful line selection and awareness of the complexity of Be-type spectra in the current measurements. Indeed given these complexities, the agreement between the two sets of measurements as shown in Fig. B2 is satisfactory.

The sample standard deviations for the $v_e \sin i$ estimates listed in Table 2 cover a large range and depend both on the quality of the spectroscopy and the degree of line broadening. Percentage errors have a smaller range and probably provide a better guide to the stochastic uncertainties. Assuming that the sample standard deviations are from a population having a normal distribution, the estimated error in the mean, $\sigma_m$, will be the sample standard deviation divided by the square root of the number of samples. In Table B3, statistics for $\sigma_m$ are summarized both for all the estimates and for those of the different quality subgroups.

For the whole sample the mean uncertainty lies in the range 3-4% with a relative narrow inter-quartile range. The subgroups with the two highest quality ratings have similar mean uncertainties and inter-quartile ranges with a maximum uncertainty of approximately 5%. By contrast, the subgroup with Q=3 has a larger mean uncertainty and inter-quartile range, with a maximum uncertainty of over 10%

In summary, the checks that we have undertaken have been encouraging. The agreement between the estimates from different lines is satisfactory and that between the two different lines sets is good. Additionally estimates obtained from the two different methodologies are consistent, whilst the agreement with previous estimates is also

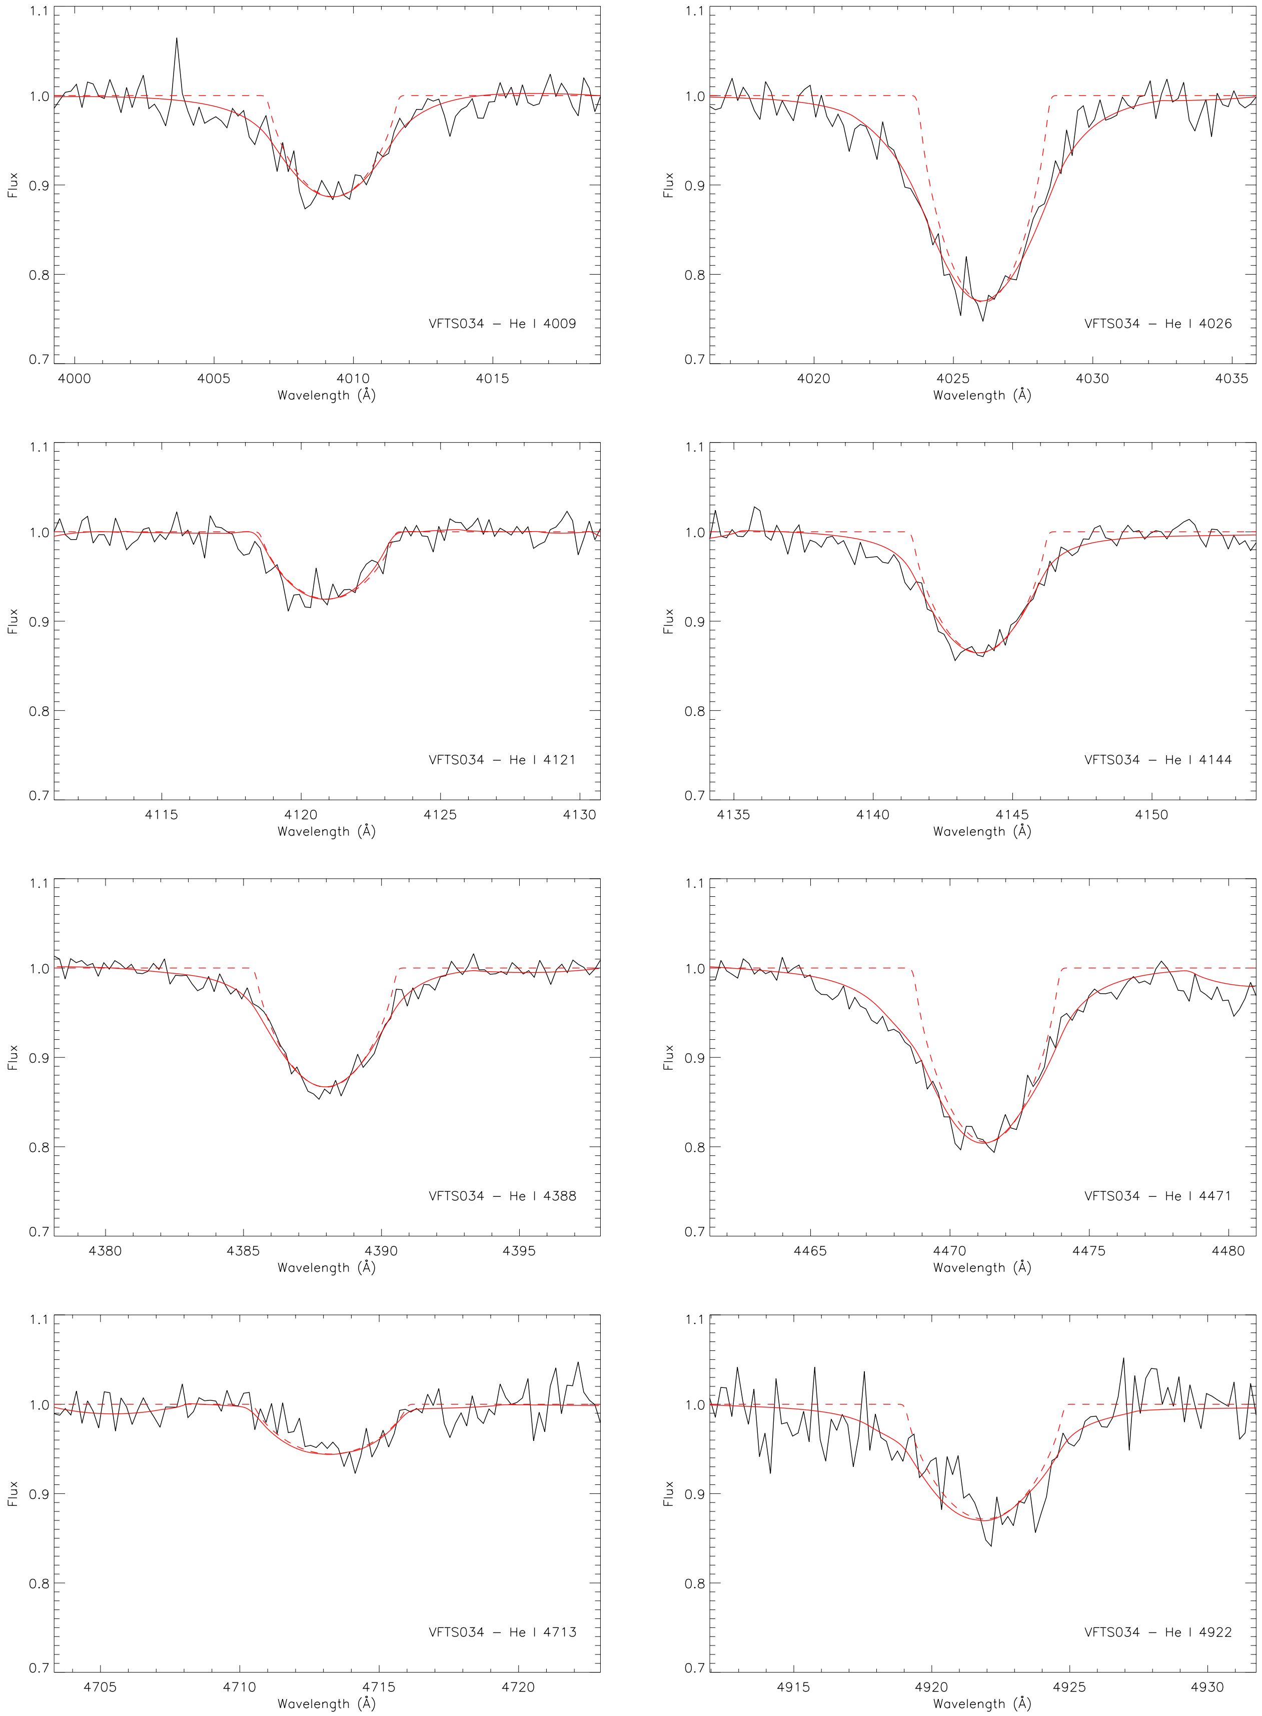


**Figure B1.** Observed and theoretical profiles for #034. The latter were for the atmospheric parameters listed in Table 4 and a microturbulence of 5 km s$^{-1}$, and have been convolved with a rotational broadening function with $v_e \sin i$= 174 km s$^{-1}$. Also shown are pure rotational broadening profiles (dotted lines) for the same $v_e \sin i$.

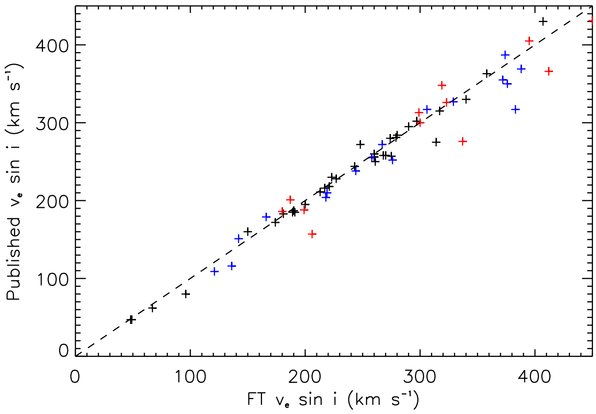


**Figure B2.** Projected rotational velocities found by Dufton et al. (2013) and Garland et al. (2017) plotted against our current Fourier Transform estimates. Black symbols have a quality rating, Q = 1, whilst blue and red symbols have Q values of 2 and 3 respectively.

**Table B3.** Statistics for the stochastic uncertainties in the $v_e \sin i$ estimates. Means, medians, inter-quartile range (IQR) and maxima are listed for the ratio of $\sigma_m$ to $v_e \sin i$, with all quantities shown as percentages.

| Sample | Mean | Median | IQR | Maximum |
|---|---|---|---|---|
| | % | % | % | % |
| All | 3.6 | 3.3 | 2.0 | 11.3 |
| Q=1 | 3.1 | 2.8 | 2.2 | 5.4 |
| Q=2 | 3.7 | 3.4 | 1.4 | 5.4 |
| Q=3 | 4.8 | 4.5 | 3.2 | 11.3 |

satisfactory. The stochastic errors in the $v_e \sin i$ estimates should be typically 3-4%, apart from the lowest quality (Q=3) measurements.

## APPENDIX C: STOCHASTIC UNCERTAINTIES IN THE $v_r$ ESTIMATES

The sample standard deviations of the radial velocity estimates range from 2–37 km s$^{-1}$, leading to estimated errors in the mean (assuming a normal distribution) ranging from 1–17 km s$^{-1}$. The latter have a median and mean of 5.4 km s$^{-1}$ and 6.2 km s$^{-1}$ respectively, with over 90% having uncertainties of less than 10 km s$^{-1}$. Hence a typical stochastic uncertainty of ±6 km s$^{-1}$ would be appropriate.

As with the projected rotational velocities estimates (see Appendix B), we can compare individual radial velocity estimates with the mean obtained for each star. For all the metal lines, systematic offsets were less than 4 km s$^{-1}$, consistent with their symmetric profiles and their utilisation for targets with relatively small projected rotational velocities. The offsets for the He I spectrum were larger and are summarized in Table C1. Two sets of offsets are provided corresponding to either the laboratory or the adopted wavelengths summarized in Table 3.

The offsets for the He I spectrum are relatively large when laboratory wavelengths are adopted, with three mean offsets being greater than 10 km s$^{-1}$. For the triplet diffuse lines these probably reflect the presence in the blue wing of a forbidden component as discussed in Sect. 4. Adopting the wavelengths from the simulation summarized in Table 3 leads to smaller offsets. Indeed for the majority of lines

**Table C1.** Differences between the $v_r$ estimates from individual He I lines and the means summarized in Table 2. The mean offsets and their standard deviations ($\sigma$) are listed both for the laboratory wavelengths and those from the simulations (see Table 3). Also listed are the number of estimates (n).

| $\lambda$ | Laboratory | | Simulations | | n |
|---|---|---|---|---|---|
| | Mean | $\sigma$ | Mean | $\sigma$ | n |
| 4009 | 7 | 16 | 5 | 16 | 49 |
| 4026 | -15 | 9 | -4 | 9 | 48 |
| 4121 | -9 | 14 | -11 | 15 | 37 |
| 4144 | 5 | 11 | -3 | 11 | 53 |
| 4388 | 15 | 17 | 9 | 17 | 52 |
| 4471 | -16 | 11 | -2 | 11 | 32 |
| 4713 | 9 | 13 | 6 | 13 | 15 |
| 4922 | 7 | 15 | 4 | 15 | 14 |

**Table C2.** Comparison of the radial velocity estimates obtained from the two line-sets. The results for Set 2 have been taken directly from Table 2. The full table is available online

| VFTS | Set 2 estimate | | | Set 1 estimate | | |
|---|---|---|---|---|---|---|
| | $v_r$ | $\sigma$ | $n$ | $v_r$ | $\sigma$ | $n$ |
| 034 | 306 | 20 | 8 | 303 | 30 | 4 |
| 166 | 267 | 14 | 8 | 288 | – | 1 |
| 194 | 280 | 13 | 6 | 291 | 4 | 2 |
| 196 | 265 | 11 | 6 | 265 | 8 | 3 |
| 200 | 260 | 9 | 7 | 256 | – | 1 |

the offsets are less than 5 km s$^{-1}$and similar to those for the metal lines. For the remaining 3 lines, the largest discrepancy is for the non-diffuse triplet at 4121 Å, which may be affected by blending with an O II line at 4119 Å; indeed this would be consistent with the lower radial velocity estimates. Removing this line would lead to an average increase of less than 2 km s$^{-1}$ in the radial velocity estimates for all the targets where it was measured.

Moderate offsets of 6–9 km s$^{-1}$ are also found for the He I lines at 4388 AA and 4713 Å. The latter is a relatively weak line and was observed in less than one quarter of the targets, with the offset not being statistically significant. That for the former is more surprising as it is well observed and apparently unblended. A relatively large offset was also found in the rotational velocity estimates from this line, although it is unclear whether these are related.

In Table C2, the radial velocity estimates from the two line-sets are compared in an analogous manner to the $v_e \sin i$ estimates in Table B2. There have a mean difference (line-set 1 - line-set 2) of 2±9 km s$^{-1}$. The overall agreement is good, whilst the standard deviations are consistent with the stochastic uncertainties discussed above.

Evans et al. (2015) have previously estimated radial velocities for 58 of our targets that were not classified as SB1.[6] Their estimates were obtained by fitting *Gaussian* profiles for a similar but more restricted sets of lines than have been considered here. In particular they did not use the He I lines at 4026 and 4471 Å. The two sets

[6] Their estimate for #272 is based on the narrow absorption lines from the nearby A-type supergiant #271 and has therefore been excluded from the comparison

of measurements are in good agreement with a mean difference (current minus Evans et al.) of -3.8±10.7 km s$^{-1}$. However, there are significant discrepancies for two targets, #298 and #467, which are discussed below. Excluding these two targets would reduce the mean difference to -2.2±6.7 km s$^{-1}$.

For #298 and #467, Evans et al. (2015) estimated radial velocities of ~330 km s$^{-1}$, considerably larger than the mean of 268±17 km s$^{-1}$found for the all VFTS B-type targets (Evans et al. 2015). By contrast, we obtained estimates of ~280 km s$^{-1}$. The reasons for these large differences are unclear but both targets have large projected rotational velocities, whilst the S/N of their spectroscopy is relatively low. Additionally there is good agreement between observed and theoretical Balmer lines profiles (see Sect. D) when we adopt the radial velocity estimates found here and this is illustrated in Fig. D2 for #298.

Observed profiles that have been Doppler shifted using the radial velocity estimates listed in Table 2 have been compared with theoretical profiles centred on the laboratory wavelengths for the metal lines and the wavelengths listed in Table 3 for the He I spectrum. The observed He I line at 4388Å on occasions appears to be redshifted relative to the theoretical profiles especially in the Q=1 targets. This is consistent with the relative large offset found for the estimates found for this line, shown in Table C1. Additionally the observed He I line at 4121Å can show an extended blue wing probably due to blending with an O II line as discussed above.

In summary, the use of our adopted He I wavelengths leads to better agreement between the radial velocity estimates from different lines. Omission of the estimates for a given feature would lead to changes in the mean that would be significantly smaller than the estimated stochastic uncertainties. Additionally there is good agreement between the estimates from the two line-sets and between the current estimates and those of Evans et al. (2015).

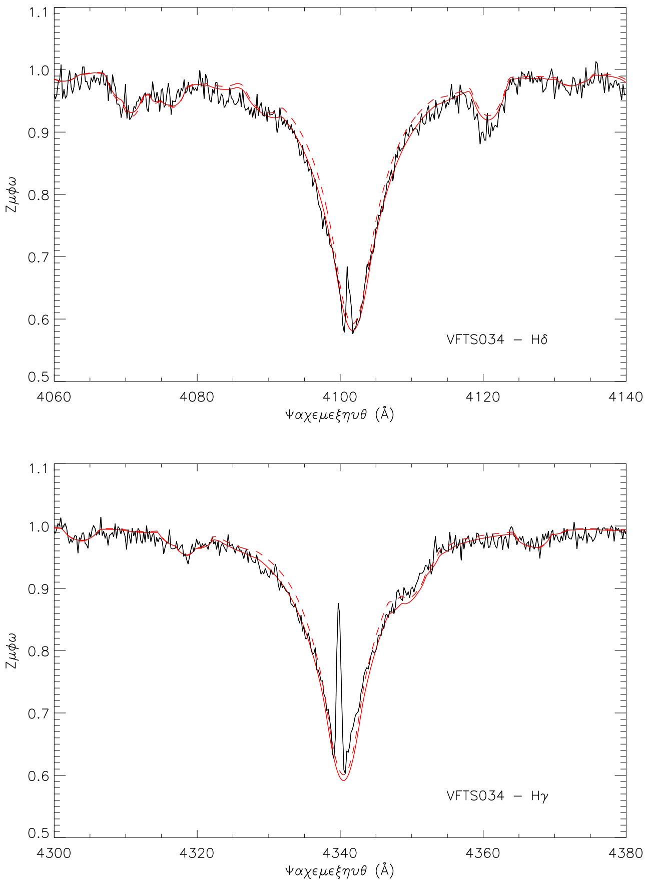


**Figure D1.** Observed and theoretical profiles for #034. The latter (solid red line) are for the atmospheric parameters listed in Table 4 and have been convoluted with a rotational broadening function using the $v_e \sin i$ estimate in Table 2. Also shown are theoretical profiles for a gravity reduced by 0.2 dex (dashed red line)

## APPENDIX D: ATMOSPHERIC PARAMETERS, STELLAR MASSES AND CRITICAL VELOCITIES

Effective temperatures, $T_{\rm eff}$ , and logarithmic surface gravities (in cm s$^-$2), log $g$ , have been estimated for all our targets. The former used the calibration of effective temperature against spectral-type for the LMC of Trundle et al. (2007), which was derived from analyses using the same model atmosphere grids as adopted here. Effective temperature estimates are listed in Table 4. For 5 targets (#030, #034, #068, #395, #486), no luminosity classification was available and $T_{\rm eff}$ estimates for a luminosity class V have been adopted. For #034 and #486, the gravity estimates discussed below are consistent with this luminosity class, whilst that for #068 would imply luminosity class III. Adopting such a classification would reduced the $T_{\rm eff}$ estimate by ~2500 K and the gravity estimate by ~0.2 dex. The other two targets (#030, #395) are discussed further below.

For some targets, the classification has a range of either spectral type and/or luminosity class. In these cases, we have taken simple averages of the values listed by Trundle et al. (2007). For example, #156 has been classified as B1-1.5 V-IIIe+ and the adopted effective temperature is the average of those predicted for B1 V, B1.5 V, B1 III, and B1.5 III. Dufton et al. (2019) estimated a typical uncertainty of 1 500K for such estimates for B-type stars in NGC 346. However given the additional complexities of Be-type spectra, the stochastic uncertainties may be larger especially for targets where the spectral type is poorly constrained.

Surface gravities were found from fitting the observed H$\gamma$ and H$\delta$ profiles. We have employed model-atmospheres calculated with the TLUSTY and SYNSPEC codes (Hubeny 1988; Hubeny & Lanz 1995; Hubeny et al. 1998; Lanz & Hubeny 2007) for a metallicity appropriate to the LMC. These non-LTE codes adopt the 'classical' stationary model atmosphere assumptions, that is plane-parallel geometry, hydrostatic equilibrium, and the optical spectrum is unaffected by winds. The grid covers a range of effective temperature, 10 000K $\leq T_{\rm eff} \leq$35 000K in steps of typically 1 500K. logarithmic gravities (in cm s$^{-2}$) range from 4.5 dex down to the Eddington limit in steps of 0.25 dex, and microturbulences are from 0–30 km s$^{-1}$ in steps of 5 km s$^{-1}$. As discussed in Ryans et al. (2003) and Dufton et al. (2005), line profiles interpolated within these grids are in good agreement with those calculated explicitly at the relevant atmospheric parameters. Further information is provided in Ryans et al. (2003), Dufton et al. (2005, 2018).

The mean difference between the estimates from the two Balmer lines was 0.00±0.10 dex with the magnitude of the differences always being ≤0.2 dex. The adopted values listed in Table 4 are the averages of those from the two Balmer lines rounded to 0.05 dex. In Figs. D1 and D2, we illustrate the quality of the fits for two target, #034 and #298. The former had relative high S/N spectroscopy, a moderate $v_e \sin i$ estimate and a quality ratio, Q=1. By contrast, the latter had lower S/N spectroscopy, the highest $v_e \sin i$ estimate in our sample,

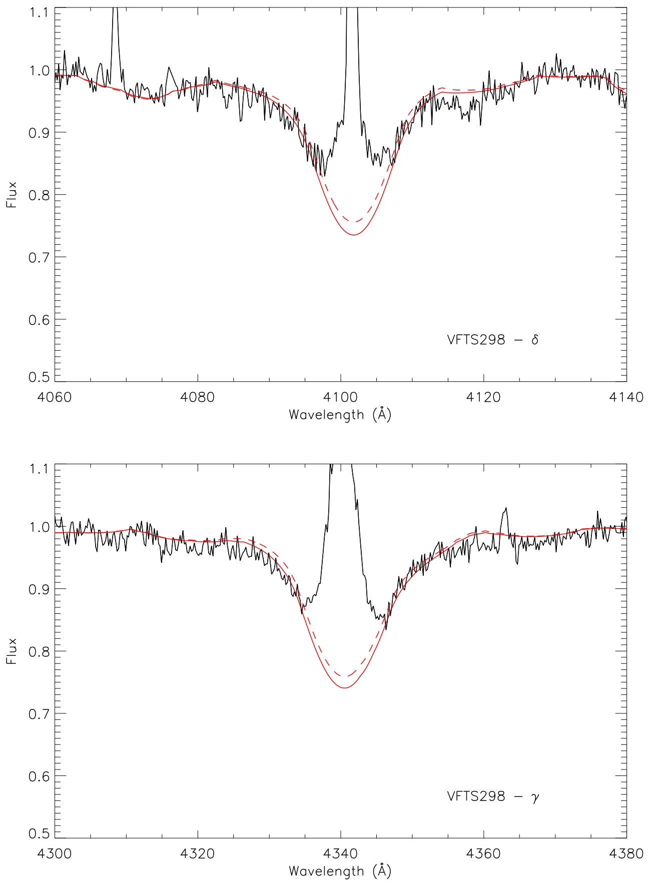


**Figure D2.** Observed and theoretical profiles for #298. The stellar parameters used to generate the latter are specified in the caption to Fig. B1. The ordinate scale has also been chosen to be the same as in Fig. D1 to aid comparison

significant emission in the Balmer line cores and a low quality rating, Q=3. As such they are representative of the range of fits achieved.

For #034, the theoretical Balmer line profiles agree well with those observed. Additionally, the O II features (at 4070-4076Å and 4035Å) and the He I doublet (at 4121Å) are well modelled, supporting the choice of atmospheric parameters. The red wing of the H$\gamma$ line implies a lower gravity possibly due to blending with a strong O II line at 4349Å and illustrates the sensitivity of the gravity estimate to the continuum normalisation. For #298, the strong emission in the line cores makes the gravity estimation more difficult although reasonable agreement between theory and observation is found in the line wings. On the basis of the quality of the fits, we adopt a stochastic uncertainty of 0.2 dex for the gravity estimates.

For most of the targets, the atmospheric parameters are consistent with their luminosity classes. Exceptions are #030, #330, #395 and #848; these have gravity estimates, $\log g < 3.2$ dex, which is beyond the limit found by Hunter et al. (2008) for hydrogen core burning objects. The last three targets have gravity estimates that lie within 0.1 dex of this limit and have luminosity classes of either III or III/II. Given the stochastic uncertainties in the gravity estimates, they may represent the lower gravity envelope of the giant population. By contrast #030 has no luminosity classification, whilst the gravity estimate of 2.75 dex is consistent with that found for luminosity class I supergiants in the VFTS survey (McEvoy et al. 2015). Additionally, whilst the He I implies a relative large $v_e \sin i$ estimate, the spectrum contains narrow metal lines, such as the Si II doublet at 4130Å, consistent with its B3-5e (shell) spectral type.

Using the atmospheric parameters estimates listed in Table 4, we have estimated current stellar masses from the grids of LMC evolutionary models of Brott et al. (2011). These have a range of initial equatorial rotational velocities, $v_i$, ranging from zero to near the critical velocity. The $v_e \sin i$ estimates for our sample has a median value of 261 km s$^{-1}$. Assuming a random distribution of inclination axes, this would translate into a median rotational velocity of $\sim$330 km s$^{-1}$(Gray 2005). We have therefore used the evolutionary models with $v_i \sim 350$ km s$^{-1}$(the actual value differs by a few km s$^{-1}$ for models with different masses). Estimates were obtained by linear interpolation between evolutionary models of different mass. Given the relative fine mesh in the model grid and uncertainties in the atmospheric parameters discussed above, this should be adequate. In Table 4, we list these estimates, rounded to the nearest solar mass.

Using these stellar parameters, we can obtain estimates of the stellar critical velocities. As discussed by Rivinius et al. (2013) misunderstandings can arise from the various definitions used when discussing critical rotation, and here we follow their definitions. Critical rotation occurs if the equatorial rotational velocity, $v_e$, reaches the Keplerian circular orbital velocity, $v_{orb}$ (hereafter designated the orbital velocity). This is given by:

$$v_{orb} = \sqrt{\frac{GM}{r_e}} \tag{D1}$$

where $r_e$ is the stellar equatorial radius.

We can also define a critical velocity, $v_{crit}$:

$$v_{crit} = \sqrt{\frac{2GM}{3r_p}} = \sqrt{\frac{2}{3}}(GMg_p)^{0.25} \tag{D2}$$

Where $g_p$ is the polar gravity and we have assumed that the polar radius ($r_p$) is relatively unaffected by rotation, The 2/3 factor above comes from the oblateness

$$r_e = \frac{3}{2} r_p \tag{D3}$$

for critical solid body rotation (see, for example, Maeder 2009).

For stars rotating at less than the critical velocity the oblateness will be smaller leading to:

$$v_{orb} \geq v_{crit} \tag{D4}$$

We can also define another velocity deduced from our mass and gravity estimates (c.f. equation D2):

$$v_c = \sqrt{\frac{2}{3}}(GMg)^{0.25} \tag{D5}$$

As our gravity estimates will the effective gravities averaged over the stellar surface, they will be lower than the polar gravity for rotating stars leading to:

$$v_{orb} \geq v_{crit} \geq v_c \tag{D6}$$

Hence these $v_c$ estimates (which are listed in Table 4) will provide lower limits to either the critical or orbital velocities.

We have investigated how uncertainties in the atmospheric parameters could affect our estimates of the critical velocity. The median effective temperature and gravity of our sample are 24 300 K and 3.6 dex. This would equate to a critical velocity of $\sim$500 km s$^{-1}$and a mass of 13 M$_\odot$. Changing the effective temperature by $\pm$1500 K would lead to corresponding changes of $\pm$15 km s$^{-1}$and $\pm$2 M$_\odot$. For the surface gravity changes by its estimated stochastic error ($\pm$0.2 dex) lead to uncertainties of $\pm^{50}_{40}$ km s$^{-1}$and $\mp$2 M$_\odot$. We adopt

typical stochastic uncertainties of ±50 km s$^{-1}$ and ±3 M$_\odot$ for our estimates of the critical velocity and stellar mass respectively.

Our atmospheric parameters assume a spatially homogeneous plane parallel geometry with no flux contamination from a disc. Frémat et al. (2005) have investigated systematic errors in the atmospheric parameters due to the former and we have adopted their results for a star with an apparent effective temperature of 24 000K and gravity of 3.8 dex. Typically the magnitude of the systematic errors increases with the inclination ($i$) of the roatation axis and increase rapidly as $\sin i \rightarrow 1$. For a star rotating at 99% of the critical velocity, the effective temperature is underestimated by 500–2500K and gravity by 0.05–0.35 dex compared with the values that would be derived if the star was not rotating. For the latter, the increase is partly a consequence of the increase in the effective temperature estimate. Decreasing the angular rotation to 80% of critical, leads to underestimates of 300–1000K and 0.02–0.30 dex respectively. Such changes in the atmospheric parameters[7] in atmospheric parameters would all lead to an underestimation of the critical velocity, with those for the gravity being potentially substantial. Indeed Zorec et al. (2016) have commented that this can lower the ratio of $v_e \sin i$ to the critical velocity when oblateness effects are included for both estimates.

The degree of flux contamination from a circumstellar disc will vary from target to target. Dunstall et al. (2011) discussed this for a sample of 31 Be-type stars in the Magellanic Clouds and found a range of disc contribution from zero to 50% of the total optical flux. For targets with significant contamination, the $T_{\rm eff}$ and $\log g$ were typically increased by ∼1 600 K and ∼0.45 dex respectively. Such changes would again lead to an increase in the estimated critical velocity with that for the gravity being potentially significant.

In summary, the atmospheric parameters must be considered with caution, given both the methodology adopted and the nature of Be-stellar spectra. Additionally given the likely systematic errors discussed above, $v_c$ estimates listed in Table 4 are best considered as lower limits to either the orbital velocity, $v_{\rm orb}$ or the critical velocity, $v_{\rm crit}$

## APPENDIX E: BIASES WITHIN THE VFTS AND NGC 346 SAMPLES

The VFTS targets were originally selected to minimise any biases, with the only constraints being a magnitude cut of V≤17.0, to ensure an adequate signal-to-noise (S/N) in the spectroscopy. For near main sequence targets, this led to both the Be-type and B-type samples having spectral types of B3 or earlier. The NGC 346 sample arises from two observational campaigns. The selection procedure for the first has been discussed by Evans et al. (2005, 2006) and involved both a magnitude and a colour cut. As Be-type stars often show additional reddening (Rivinius et al. 2013) this could have led to the exclusion of some Be-type stars. Additionally known Be-type stars were excluded for the observation of some Magellanic Cloud clusters but this did not affect the target selection for NGC 346. The selection procedure for the second campaign has been discussed in Dufton et al. (2019) and employed similar magnitude and colour cuts. If the inclusion of a colour cut was a significant source of bias, Be-type stars would be expected to be under-represented in the NGC 346 sample compared to the VFTS sample. In fact, the reverse appears to be the case implying that this cannot explain the different ratios. The magnitude limits again led to the NGC 346 samples having a similar range of spectral types to those for the VFTS samples.

Be-type stars may be over-luminous for their spectral type (see, for example, Townsend et al. 2004; Rivinius et al. 2013; Zorec et al. 2016, and references therin). If this over-luminosity is principally due to rotation, a similar offset in luminosity would be expected in the rapidly rotating B-type stars. However if it principally arose from the Be-type phenomena (such as the circumstellar environment), it could lead to a bias towards Be-type stars in both samples.

The two observational samples also sample different environments and stellar ages. The VFTS observations were all located within the Tarantula nebula, with a relatively large percentage of targets associated with clusters. Schneider et al. (2018b) discuss the star formation history of 30 Doradus and concluded that massive star formation rapidly accelerated about 8 Myr ago and then diminished 1Myr ago. By contrast, the compact nature of NGC 346 leads to the dataset being strongly weighted towards field stars. For example only 20% of the apparently single B- and Be-type stars lie within 2′ of its centre, whilst the median age of the apparently single B-type stars is 13 million years (Dufton et al. 2019).

The Be-type stars make up 22% and 28% of the non-supergiant apparently single B-type targets for the VFTS and NGC 346 survey respectively. A Pearson $\chi^2$ test yield a P-value of 11.5% that the two datasets sampled the same Be-type population.

This paper has been typeset from a TEX/LATEX file prepared by the author.

[7] an increase in the adopted gravity will lead to a decrease in the stellar mass estimate. However the overall effect is still an increase in the critical velocity estimate
